# Supplementary material for: Manipulating and Measuring Model Interpretability
Source: arXiv:1802.07810 source file (2021-08-15)
Supplement: Supplementary file 1 [file exp1_instructions.pdf]

# Instructions

**!! IMPORTANT !! Your session will expire in 60 minutes. Please make sure to complete the HIT in 60 minutes!**

---

- You are here to predict **New York City apartment prices in the Upper West Side** with the help of a model.
  - There will be a training.phase and a testing.phase:
    - In the training phase, you will see examples of apartments along with what the model predicted they sold for and the actual price they sold for.
    - In the testing phase, you will see new apartments and make your own prediction about what the model will predict and what the actual price is.
- 

Next ➡

# Instructions

---

- You will see these properties for each apartment:

| Properties              |       |
|-------------------------|-------|
| # Bedrooms              | 2     |
| # Bathrooms             | 2     |
| Square footage          | 1140  |
| Total rooms             | 6     |
| Days on the market      | 47    |
| Maintenance fee (\$)    | 811   |
| Subway distance (miles) | 0.122 |
| School distance (miles) | 0.278 |

---

[← Previous](#)

[Next →](#)

# Instructions

- A model predicts apartment prices. We will explain how this model works in the next page.
  - This model uses # Bathrooms and Square footage of the apartment to make its prediction.
  - The graph at the bottom shows this price visually.

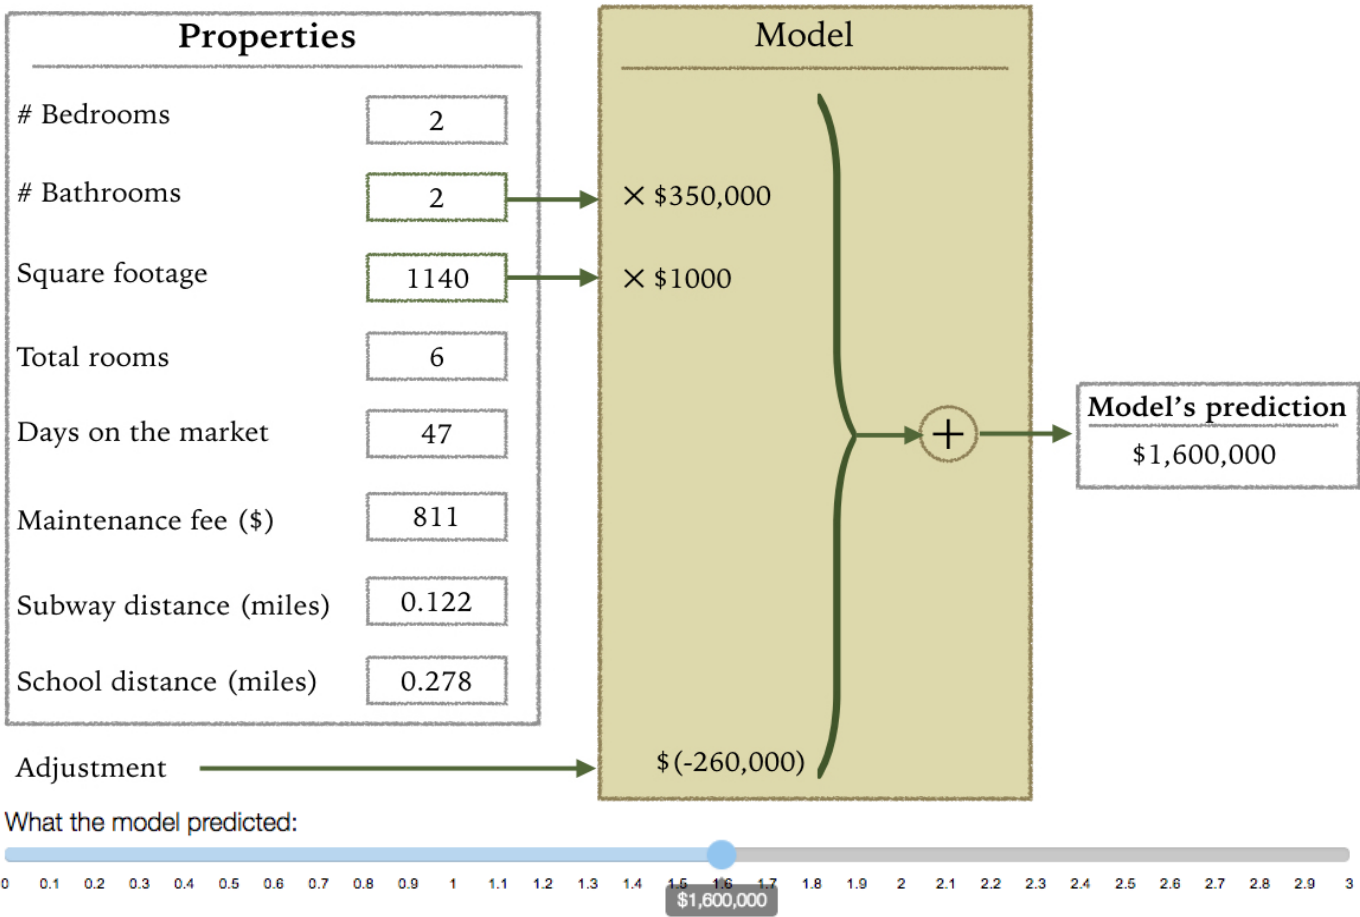

← Previous

Next →

# Instructions

- Here is how the model has made its prediction:
- Each bathroom is worth \$350,000. Therefore, \$350,000 is multiplied by the number of bathrooms and added to the price. This is repeated for Square footage. Finally, **the adjustment factor of \$260,000 is subtracted** and a price is predicted.

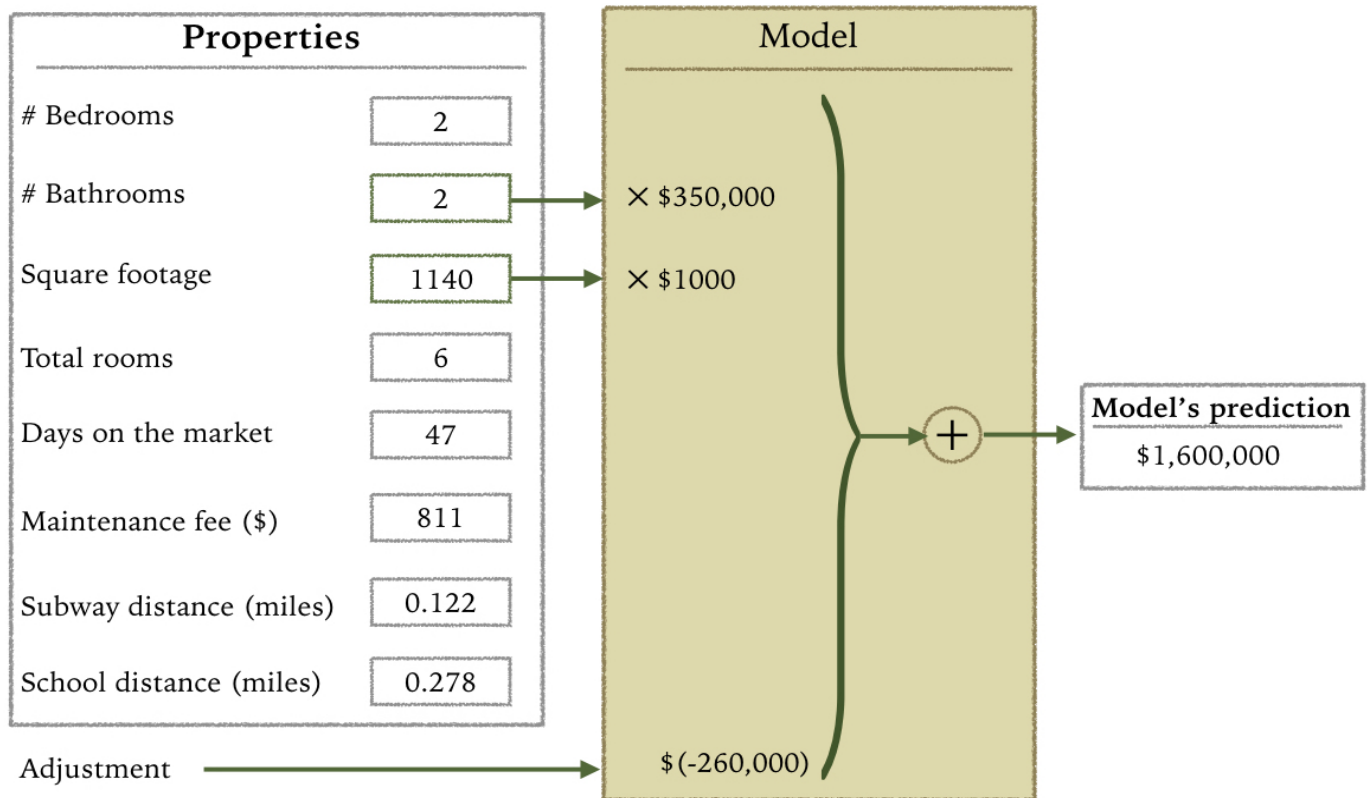

$$\begin{aligned} & [2 \times 350,000] + [1140 \times 1000] + [-260,000] \\ & \underbrace{\hspace{1cm}} \quad \underbrace{\hspace{1cm}} \quad \underbrace{\hspace{1cm}} \\ & 700,000 \quad + \quad 1,140,000 \quad + \quad [-260,000] \\ & \approx 1,600,000 \end{aligned}$$

← Previous

Next →

# Training Phase Instructions

---

- There will be ten apartments in the training phase.
- For each apartment, you will complete the following two steps:

---

[← Previous](#)

[Next →](#)

# Training Phase Instructions-Step 1

Properties

# Bedrooms

2

# Bathrooms

2

Square footage

1140

Total rooms

6

Days on the market

47

Maintenance fee (\$)

811

Subway distance (miles)

0.122

School distance (miles)

0.278

Model

×

\$350,000

×

\$1000

+

Model's prediction

\$1,600,000

Adjustment

→

\$(-260,000)

What the model predicted:

0

0.1

0.2

0.3

0.4

0.5

0.6

0.7

0.8

0.9

1

1.1

1.2

1.3

1.4

1.5

1.6

1.7

1.8

1.9

2

2.1

2.2

2.3

2.4

2.5

2.6

2.7

2.8

2.9

3

\$1,600,000

What do you think this apartment actually sold for?

0

0.1

0.2

0.3

0.4

0.5

0.6

0.7

0.8

0.9

1

1.1

1.2

1.3

1.4

1.5

1.6

1.7

1.8

1.9

2

2.1

2.2

2.3

2.4

2.5

2.6

2.7

2.8

2.9

3

\$0

← Previous

Next →

# Training Phase Instructions-Step 2

- In step 2, you will see what this apartment actually sold for and how you and the model did:
- There are three graphs at the bottom:
  - The first graph shows the model's prediction of the price of this apartment.
  - The second graph shows what you thought this apartment actually sold for.
  - The third graph shows what this apartment actually sold for.

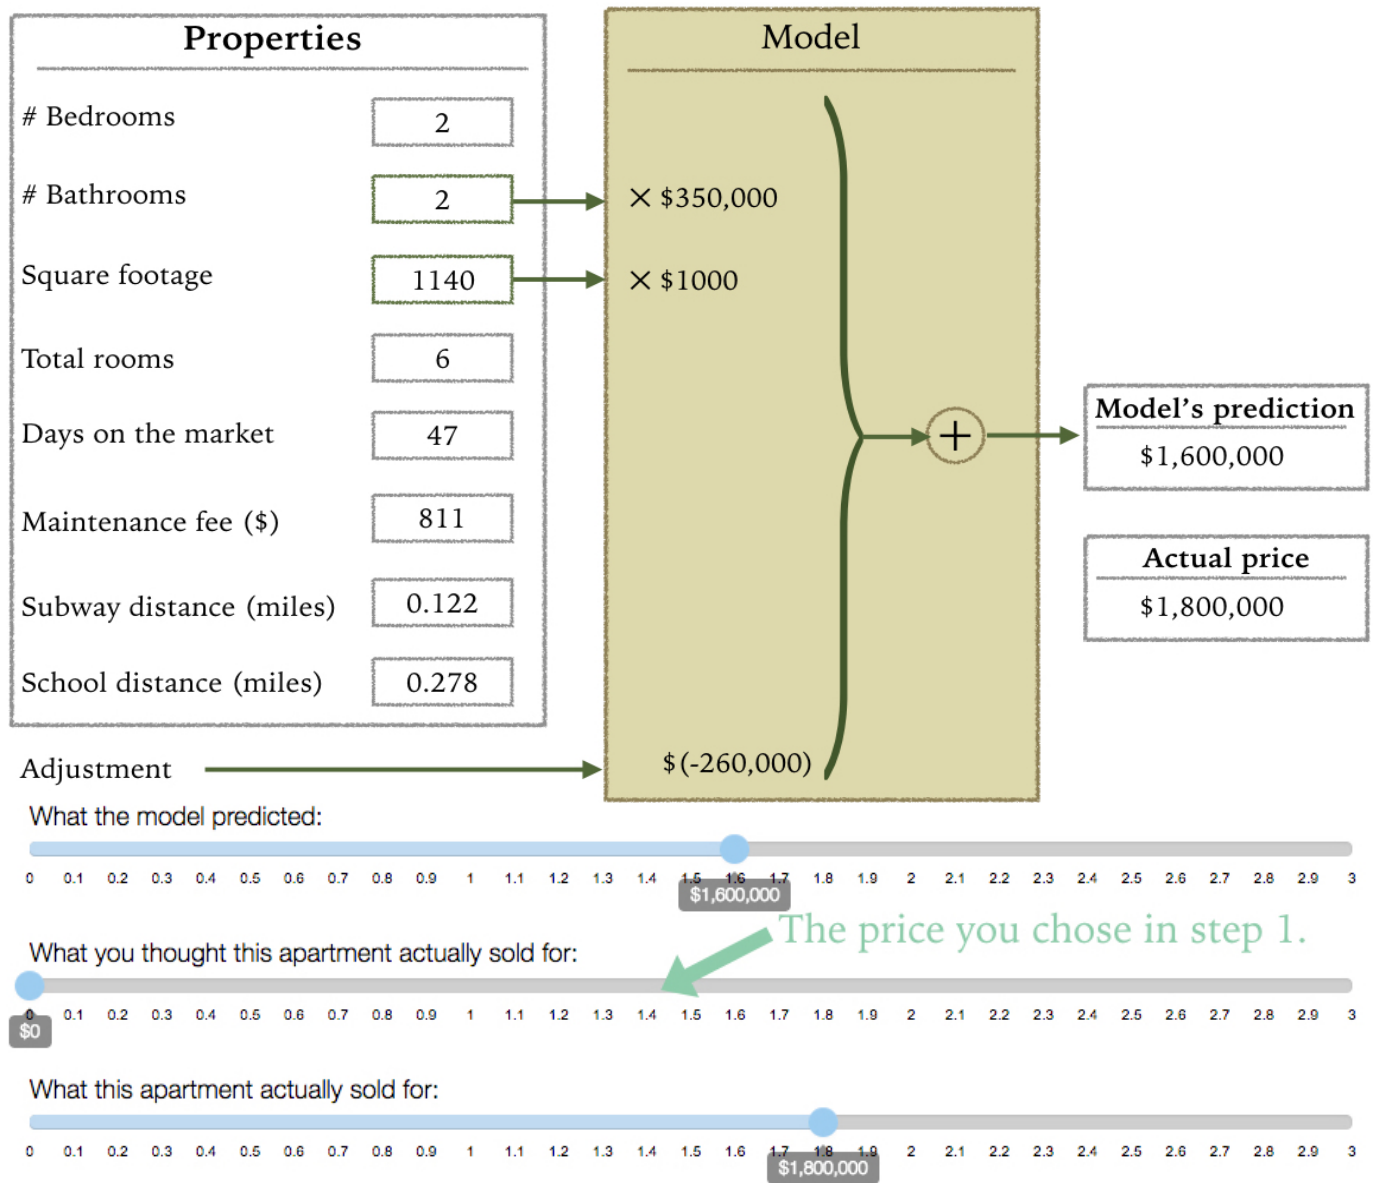

# Instructions

---

- Once you have reviewed all ten apartments in the training.phase, you will move to the testing.phase.
- In the testing phase, you will see twelve new apartments and you will guess the price each was sold for.
- **NOTE:** You will not see the actual prices for these apartments in the testing phase. Once you are done, you will see how you did overall.
- For each apartment, you will complete the following three steps:

---

← Previous

Next →



# Testing Phase Instructions-Step 1

- In step 1, you will state what you think the model will predict and how confident you are that the model will make that prediction:

Properties

# Bedrooms

1

# Bathrooms

1

Square footage

841

Total rooms

3.5

Days on the market

36

Maintenance fee (\$)

505

Subway distance (miles)

0.122

School distance (miles)

0.278

Model

× \$350,000

× \$1000

+

\$(-260,000)

Adjustment

What do you think the model will predict?

0

0.1

0.2

0.3

0.4

0.5

0.6

0.7

0.8

0.9

1

1.1

1.2

1.3

1.4

1.5

1.6

1.7

1.8

1.9

2

2.1

2.2

2.3

2.4

2.5

2.6

2.7

2.8

2.9

3

\$800,000

How confident are you the model will predict this?

1

2

3

4

5

It's likely the model will predict something else

I'm confident the model will predict this

← Previous

Next →

# Testing Phase Instructions-Step 2

- In step 2, you will see what the model predicts and you will state how confident you are that the model made the right prediction:

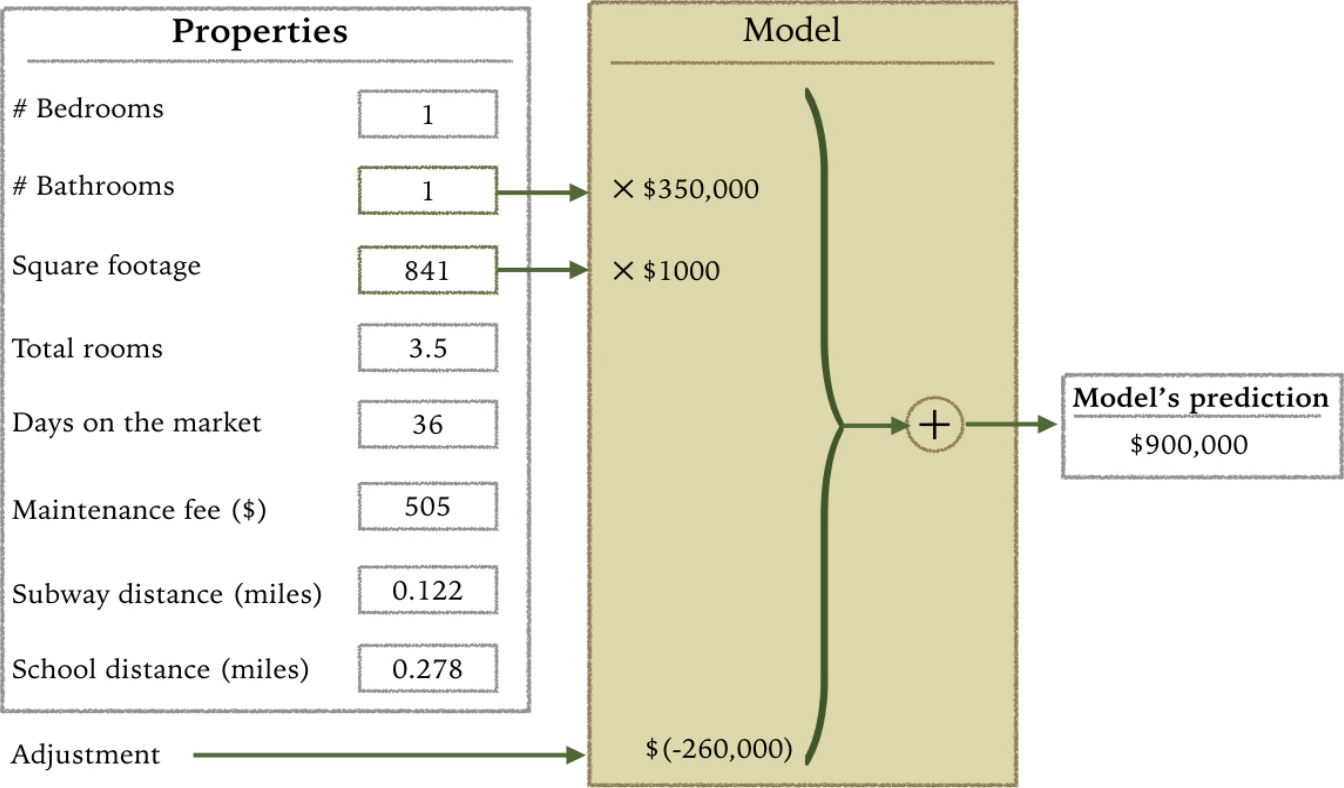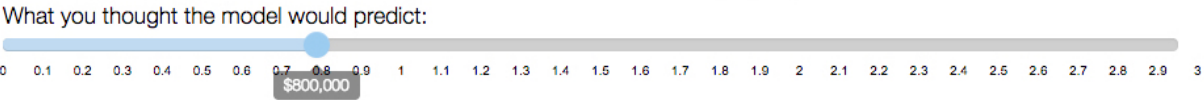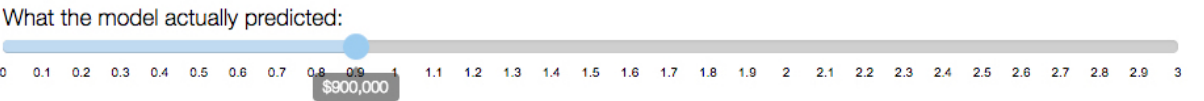

How confident are you that the model got it right?

1 2 3 4 5

I'm confident the model got it wrong ☐ ☐ ☐ ☐ ☐ I'm confident the model got it right

← Previous

Next →

# Testing Phase Instructions-Step 3

- In step 3, given the model's prediction, you will state what you think this apartment actually sold for and your confidence:

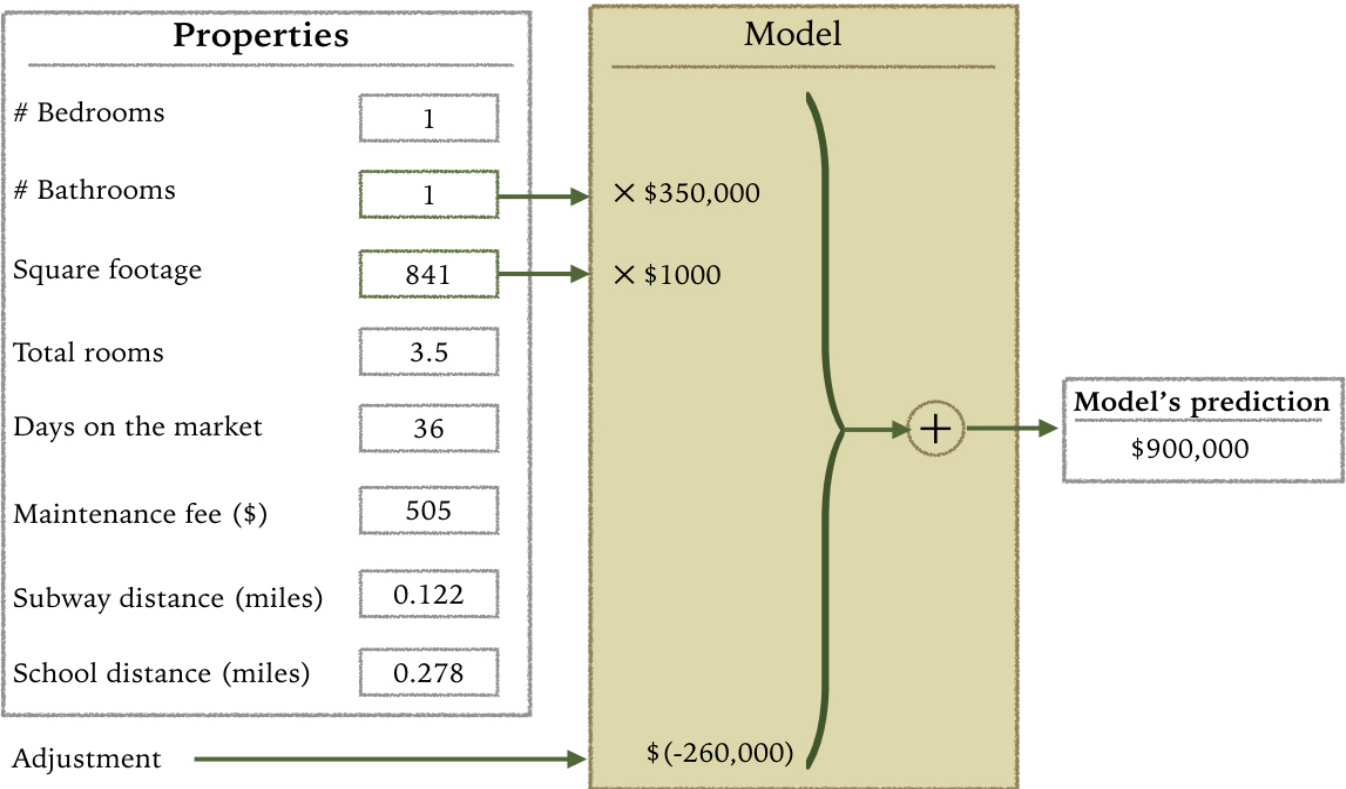

What you thought the model would predict:

0 0.1 0.2 0.3 0.4 0.5 0.6 0.7 0.8 0.9 1 1.1 1.2 1.3 1.4 1.5 1.6 1.7 1.8 1.9 2 2.1 2.2 2.3 2.4 2.5 2.6 2.7 2.8 2.9 3

\$800,000

What the model actually predicted:

0 0.1 0.2 0.3 0.4 0.5 0.6 0.7 0.8 0.9 1 1.1 1.2 1.3 1.4 1.5 1.6 1.7 1.8 1.9 2 2.1 2.2 2.3 2.4 2.5 2.6 2.7 2.8 2.9 3

\$900,000

What do you think this apartment actually sold for?

0 0.1 0.2 0.3 0.4 0.5 0.6 0.7 0.8 0.9 1 1.1 1.2 1.3 1.4 1.5 1.6 1.7 1.8 1.9 2 2.1 2.2 2.3 2.4 2.5 2.6 2.7 2.8 2.9 3

\$0

How confident are you that you got it right?

1 2 3 4 5

It's likely I got it wrong

I'm confident I got it right

# Instructions

---

- Once you are done with twelve apartments in the testing phase, you will see your results and how you did overall.
- You are now done with all the instructions. Thanks for participating in this experiment!

**You must provide correct answer to the following question to proceed:**

---

Each apartment has the following 8 properties:

# Bedrooms, # Bathrooms, Square footage, Total rooms, Days on the market, Maintenance fee, Subway distance, and School distance

How many of these apartment properties does the model use to make its prediction?

- ☐ 1 property
- ☐ 2 properties
- ☐ 3 properties
- ☐ 4 properties
- ☐ 5 properties
- ☐ 6 properties
- ☐ 7 properties
- ☐ 8 properties

Submit

---

← Previous

Next →

# Starting the Training Phase...

---

- You will now start the training phase.
- You will see ten apartments, the price that the model predicted, and the price that they were actually sold for.
- Pay attention to apartment properties and how they relate to the actual price and the model's prediction.
- **You won't be able to go back to the training phase once you get to the testing phase!**

---

← Previous

Begin training phase →
